# Supplementary material for: FedMoE: Personalized Federated Learning via Heterogeneous Mixture of Experts
Source: arXiv:2408.11304 source file (2024-08-21)
Supplement: Supplementary file 1 [file sec-appendix.tex]

\newpage
\appendix

\section{Appendix A: Experimental Details}
\subsection{Computing Infrastructure}
The computing infrastructure for conducting the experiments is as follows:

\textbf{Hardware Environment}: The servers are equipped with NVIDIA A800 GPUs, each with 80GB of VRAM, and Intel Xeon Silver CPUs. The systems include 1 TB of system memory.

\textbf{Software Environment}: The operating system in use is CentOS Linux 7 (Core). The software stack includes the PyTorch framework (version 1.12.1+cu113), Hugging Face’s transformers library (version 4.35.2), and the adapters library from AdapterHub (version 0.1.0).

\subsection{Hyperparameters}
For all FL methods, we set the training and validation batch sizes to 16. A random seed of 42 was used for experiment reproducibility. The local training epoch is set to 1, and the entire federated learning process lasts for 100 rounds. \sys{} is optimized using the Adam optimizer with a learning rate of $1e-4$, which is the optimal choice within the range of $1e-5$ to $1e-3$. For the first stage of \sys{}, the edge devices only perform a quick fine-tuning for 5 epochs, which is sufficient to reveal the patterns for expert activations. The memory threshold coefficient $\alpha$ for heuristic search is set to 0.75 to ensure the performance of initialized models while avoiding excessive memory usage. For the second stage of \sys{}, the number $K$ of clients participating in expert recommendation is set to 3.
% seq length, acc not imporve for 1 epoch

We run each FL method three times and report the
average results.
\section{Appendix B: Further Discussion}
To provide a comprehensive understanding of the system's performance, we further discuss the results of submodel initialization, submodel adjustment and the final activation patterns for \sys{}.

\begin{figure}[htbp]
    \centering
    \includegraphics[width=0.8\linewidth]{C:/Users/12085/Desktop/FedMoE-AAAI-LaTeX/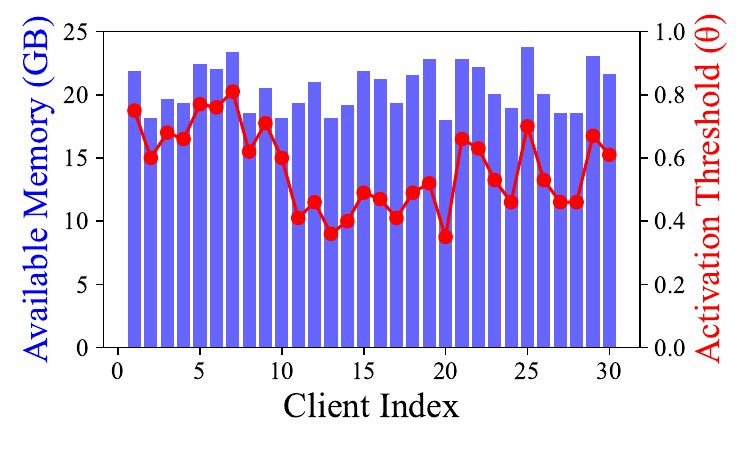}
    \caption{Memory capacities and activation thresholds across clients.}
    \label{fig:memory_theta}
\end{figure}
Figure~\ref{fig:memory_theta} reveals the results of the heuristic search for various clients in the first stage of \sys{}. Generally, clients with larger memory capacity tend to set higher activation threshold, thereby retaining a greater number of experts. This strategy effectively optimizes resource usage while maintaining model performance. However, the relationship between activation threshold and memory capacity is non-linear, as the setting of activation threshold is also influenced by factors such as data distribution, task types, and the performance of individual experts.

\begin{figure}[htbp]
    \centering
    \includegraphics[width=0.8\linewidth]{C:/Users/12085/Desktop/FedMoE-AAAI-LaTeX/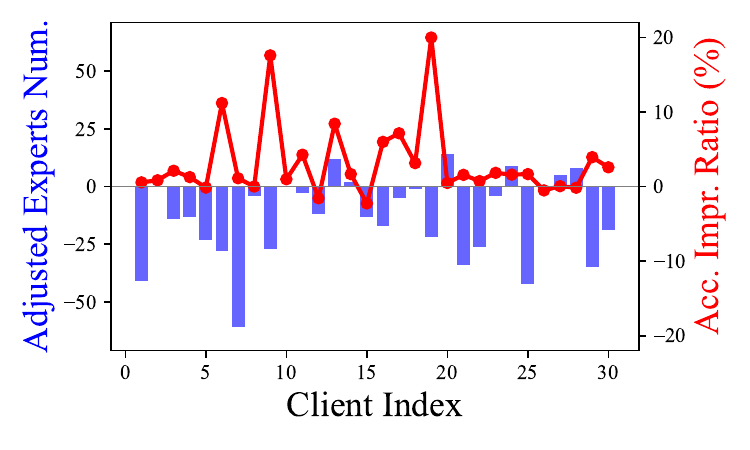}
    \caption{Number of adjusted experts and accuracy improvements across clients.}
    \label{fig:acc_improve}
\end{figure}
Figure~\ref{fig:acc_improve} illustrates the results of submodel adjustments in the second stage of \sys{}. 68.75\% of clients tend to prune redundant experts, indicating that the system effectively adjusts towards resource efficiency. After fine-grained adjustments, 84.38\% of the submodels demonstrate improved performance, indicating that the submodels transition from suboptimal to optimal.

\begin{figure}[htbp]
    \centering
    \includegraphics[width=0.8\linewidth]{C:/Users/12085/Desktop/FedMoE-AAAI-LaTeX/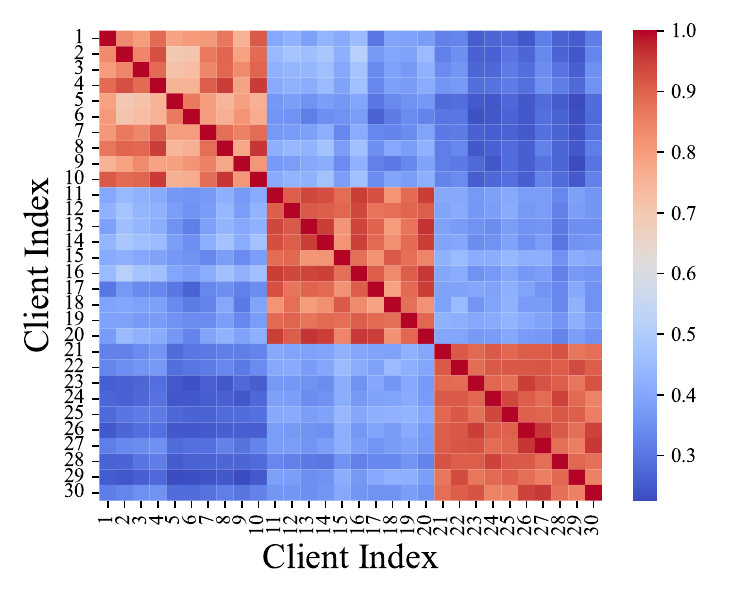}
    \caption{Similarity of activation pattern across clients.}
    \label{fig:similarity}
\end{figure}
Figure~\ref{fig:similarity} illustrates the similarity in expert activation probabilities between client pairs after training, where clients 1-10, 11-20, and 21-30 each handle the same type of task. The red areas on the heatmap indicate that clients with the same task are likely to activate similar subsets of experts, which facilitates mutual enhancement of expertise. There are still variations among these clients due to different data distribution and resource availability. The blue areas show low similarity between clients with different types of tasks, reducing interference among experts and ensuring the model's versatility across various task types. This differentiated expert activation pattern equips the model with better task-specific knowledge, thereby optimizing performance in cross-task scenarios.

% \begin{figure}[htbp]
%     \centering
%     \includegraphics[width=0.5\linewidth]{C:/Users/12085/Desktop/FedMoE-AAAI-LaTeX/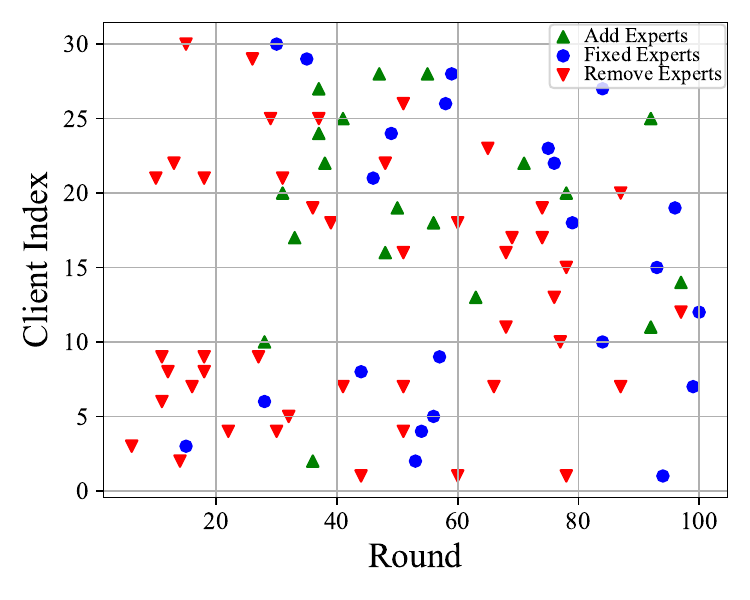}
%     \caption{Caption describing the image.}
%     \label{fig:decision_map}
% \end{figure}
